# Supplementary material for: Likelihood-Based Heterogeneity Inference Reveals Non-Stationary Effects in Biohybrid Cell-Cargo Transport
Source: arXiv:2508.12976 ancillary file (2026-02-03)
Supplement: Supplementary file 1 [file main_SI.pdf]

# SUPPLEMENTAL MATERIAL

## Likelihood-Based Heterogeneity Inference Reveals Non-Stationary Effects in Biohybrid Cell-Cargo Transport

Jan Albrecht, Lara S. Dautzenberg, Manfred Opper, Carsten Beta, Robert Großmann

### S1 Experimental setup

The experimental setup is identical to the one presented in Ref. [2].

*Dictyostelium discoideum* cells of the AX2-214 wild-type strain were cultured in untreated polystyrene cell culture flasks (T-75 Standard, Sarstedt AG & Co. KG, Nümbrecht, Germany) in 10 ml *HL5* medium including glucose (Formedium Ltd. Norfolk House, Norfolk, England), supplemented with 100 units/ml Penicillin G sodium salt and 0.1 mg/ml Streptomycin sulfate (Penicillin- Streptomycin 10X Solution, Biological Industries, Beit Haemek, Israel) at 21°C. The growth medium was exchanged every two to three days. The cells were diluted regularly to avoid confluency. The cell culture was renewed every 4 weeks at the latest.

In preparation for the experiments, the cells were harvested and suspended in fresh nutrient medium. The cell density was adjusted to  $1 \cdot 10^6$  cells/ml. The experiment was performed using a chambered coverslip with individual wells and an imprinted  $500 \mu\text{m}$  location grid (ibidi GmbH, Gräfelfing, Germany) with  $1.0 \text{ cm}^2$  of growth area per well.  $298 \mu\text{l}$  of the prepared cell suspension was transferred to each of the wells leading to a cell density of about 30 cells per  $100 \mu\text{m} \times 100 \mu\text{m}$ . The cells were given 20 min to sediment and attach to the bottom of the wells.

As cargo, monodispersed spherical polystyrene beads were used (microParticles GmbH, Berlin, Germany). 20 min after the cells had been introduced into the wells,  $2 \mu\text{l}$  of bead suspension (for concentration see table below) were added in each well just below the surface of the nutrient medium. The slide was slightly tilted to distribute particles as evenly as possible. The concentration of the beads in the suspension was chosen to strike a balance between a high number of recorded beads and a low number of bead collisions. The measurements were started between 20 and 60 minutes after adding the polystyrene beads.

The experiments were carried out with 4 different bead sizes:

| diameter [ $\mu\text{m}$ ] | standard deviation [ $\mu\text{m}$ ] | concentration of<br>bead suspension [ $10^3 \cdot \mu\text{l}^{-1}$ ] | referred to as    |
|----------------------------|--------------------------------------|-----------------------------------------------------------------------|-------------------|
| 29.32                      | 0.25                                 | 0.36                                                                  | 29 $\mu\text{m}$  |
| 46.30                      | 0.37                                 | 0.32                                                                  | 46 $\mu\text{m}$  |
| 61.6                       | 1.1                                  | 0.30                                                                  | 61 $\mu\text{m}$  |
| 101.0                      | 1.6                                  | 0.16                                                                  | 100 $\mu\text{m}$ |

The main text presents the data from the 61  $\mu\text{m}$  experiments. The results for the remaining sizes are shown in Sec. S3 of this supplement.

The images were taken with an OLYMPUS XM10 CCD camera (OLYMPUS XM10, resolution:  $1376 \times 1032$  pixels, 8 bit grey scale) through an OLYMPUS IX71 bright field microscope (Olympus Deutschland

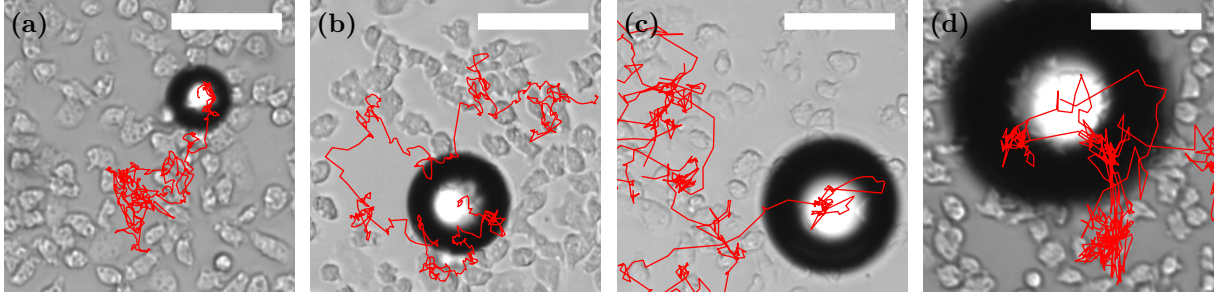

**Figure S1:** Exemplary cropped frames of selected beads with superimposed tracked trajectories. The scale bar has a width of  $50\,\mu\text{m}$ . The four images show different bead diameters: (a)  $29\,\mu\text{m}$ , (b)  $46\,\mu\text{m}$ , (c)  $61\,\mu\text{m}$ , (d)  $100\,\mu\text{m}$ . For  $61\,\mu\text{m}$  and  $100\,\mu\text{m}$  only part of the trajectory is visible. In every case the image is the last one of the respective recording.

GmbH, Hamburg, Germany) with a 10x objective (Olympus UPLanFL N 10x/0.30na). An image was taken every 15 s for a total duration of 4 hours. An exposure time of ten milliseconds was set. Using a computer controlled motorized stage (Märzhäuser Wetzlar GmbH & Co. KG, Wetzlar, Germany), several different positions were recorded during a single run of the experiment. The focal plane was adjusted such that polystyrene particles appeared as black circles with a bright spot in the middle. Figure S1 shows exemplary cropped frames with the tracked trajectories (see Sec. S2) superimposed.

## S2 Data processing

The images captured by the microscopy setup were processed using a custom Matlab code. Using the location grid of the wells as fixed points, a stage correction was performed to remove any jitter from small inaccuracies of the stage placements. After this correction, the images were cropped to exclude the grid since the grooves of the grid might influence the cell behavior. After that, the positions of the bead centroids were tracked and combined into bead trajectories. Touching beads were not tracked; a collision of two beads ended each of their tracked trajectories. A circularity criterion was defined that excluded beads with insufficient area within the frame. Camera or stage errors could lead to individual positions missing from the dataset. Such an error occurred about once every 1000 images. Similarly, there are missing positions in the trajectory of a bead which temporarily ( $\leq 3$  frames) violated the circularity criterion due to its proximity to a frame boundary. The number of trajectories  $N$  for each of the datasets is given in the following table; an overview over the trajectory length distributions is given in Fig. S2:

|                    | $N$ |
|--------------------|-----|
| $29\,\mu\text{m}$  | 266 |
| $46\,\mu\text{m}$  | 189 |
| $61\,\mu\text{m}$  | 177 |
| $100\,\mu\text{m}$ | 80  |

Except for the  $100\,\mu\text{m}$  dataset, trajectories that (almost) last the full time of the experiment are most common.

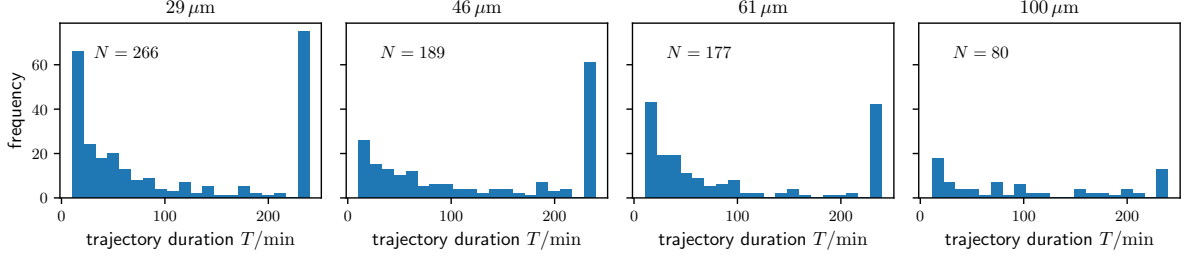

**Figure S2:** Trajectory duration distribution of the recorded particle trajectories. The total recording time was four hours.

### S3 Results for additional bead sizes

In Figs. S3-S6 we report the results of the analysis in the main text for all four datasets with different bead sizes. For the convenience of the reader we have also included here again the results for the  $61\ \mu\text{m}$  beads that have already been presented in the main text. The figure captions are intentionally kept concise. For more details see the corresponding figure captions of the main text. Here we discuss the most important points of this comparative analysis.

The preliminary statistical analysis of the datasets yields very similar results to the one studied in the main text. The *eamsd* as well as the *eatamsd* is linear (see sub-panels (a)) and non-overlapping bead displacements with interval lengths  $\tau$  above 2 min are independent (see sub-panels (b)). For the  $100\ \mu\text{m}$  beads this is even true for interval lengths down to just 30 seconds. Closer inspection of the *eatamsd* curves reveals that the crossover time at which the *eatamsd* goes from super-linear to linear is smaller the larger the bead size. In all cases the step-size distributions have non-Gaussian tails (see sub-panels (c)). The histograms of the single trajectory estimates  $\hat{\sigma}^2$  are well approximated by a  $\Gamma$ -distribution (see sub-panels (e)). Therefore, we can use the same motility and heterogeneity model as in the main text for the other datasets as well.

For all datasets there are several trajectories with a wide range of plausible values of the noise strength  $\sigma^2$  with respect to the width of the distribution of noise strengths over the whole dataset (see sub-panels (d)). Except for the  $100\ \mu\text{m}$  dataset, the estimate obtained from the two level approach is outside the uncertainty bounds of the Bayes estimate (see sub-panels (f)). Note that the average noise strength (which is proportional to the diffusion constant) of the beads increases very significantly with the bead diameter (see sub-panels (e) and (i)).

We now consider the temporal change of the heterogeneity within the data. In the datasets for  $46\ \mu\text{m}$ ,  $61\ \mu\text{m}$ , and  $100\ \mu\text{m}$  beads the mean as well as the variance of the distribution is significantly larger during the first two hours than during the second two hours of the experiment (see sub-panels (i)). In case of the  $100\ \mu\text{m}$  dataset there are strong fluctuations which are probably due to the low number of total trajectories in this dataset. In the  $46\ \mu\text{m}$  dataset we can see a stabilization of the heterogeneity in the second half of the experiment just as for the  $61\ \mu\text{m}$  dataset discussed in the main text. The discussion about the shift in heterogeneity presented in the main text also applies here.

The picture about the shift of heterogeneity in the  $29\ \mu\text{m}$  dataset is less clear than for the other bead diameters. A possible explanation could be that the small size of the beads which is on the order of two cell diameters leads to different interaction dynamics between cells and beads. Ameboid cells are known to sense curvature [3] and might react differently when encountering objects with a size similar to their

own. Furthermore the accumulation effect will be less pronounced since only few cells can be in contact with a single bead at any given time.

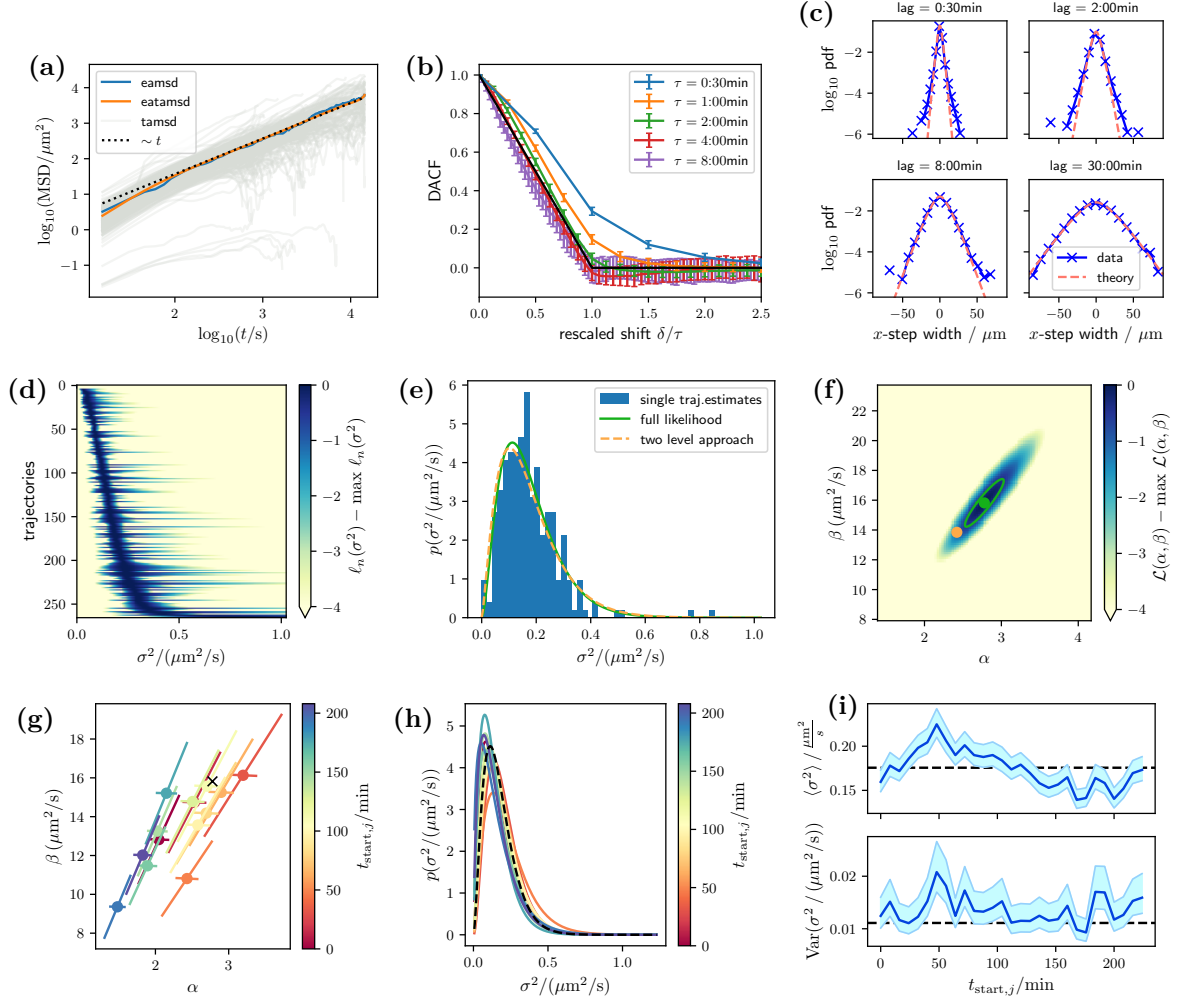

**Figure S3:** Results for dataset with bead diameter of  $29 \mu\text{m}$ . The inference results are obtained using sparse versions of the trajectories with  $\Delta t = 2 \text{ min}$ . The first row shows the preliminary statistical analysis: (a) mean squared displacement, (b) normalized and rescaled displacement autocorrelation function, (c) step-size distributions. The second row shows inference using the full length of each trajectory: (d) single trajectory log-likelihood of  $\sigma^2$ , (e) distribution of single trajectory estimates and inferred heterogeneity, (f) log-likelihood of the heterogeneity parameters. The third row shows results of heterogeneity inference using data within a time window of 16 min: (g) inferred heterogeneity parameter, (h) inferred probability density functions, (i) mean and variance of the inferred distributions.

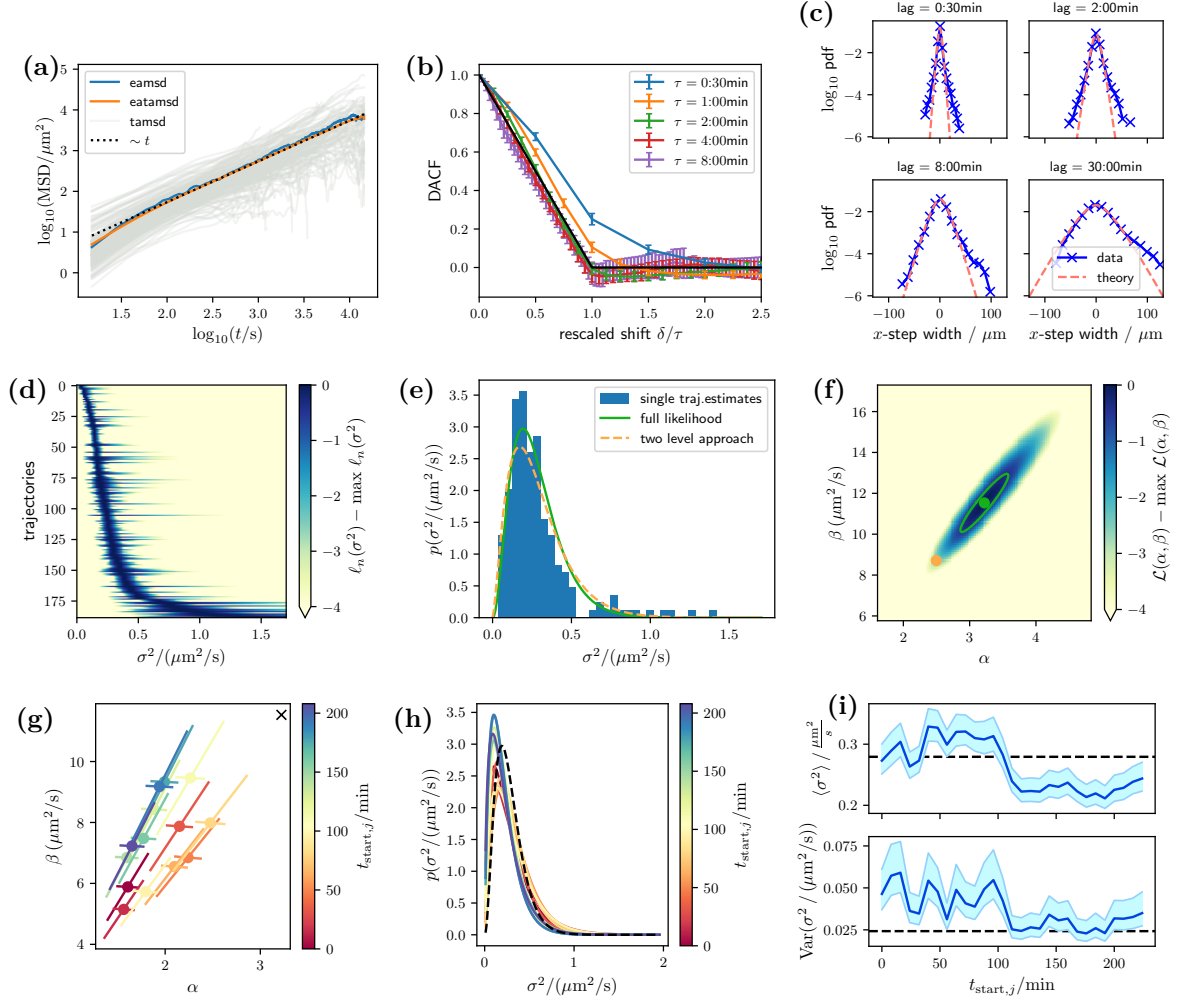

**Figure S4:** Results for dataset with bead diameter of  $46 \mu\text{m}$ . The inference results are obtained using sparse versions of the trajectories with  $\Delta t = 2 \text{ min}$ . The first row shows the preliminary statistical analysis: (a) mean squared displacement, (b) normalized and rescaled displacement autocorrelation function, (c) step-size distributions. The second row shows inference using the full length of each trajectory: (d) single trajectory log-likelihood of  $\sigma^2$ , (e) distribution of single trajectory estimates and inferred heterogeneity, (f) log-likelihood of the heterogeneity parameters. The third row shows results of heterogeneity inference using data within a time window of 16 min: (g) inferred heterogeneity parameter, (h) inferred probability density functions, (i) mean and variance of the inferred distributions.

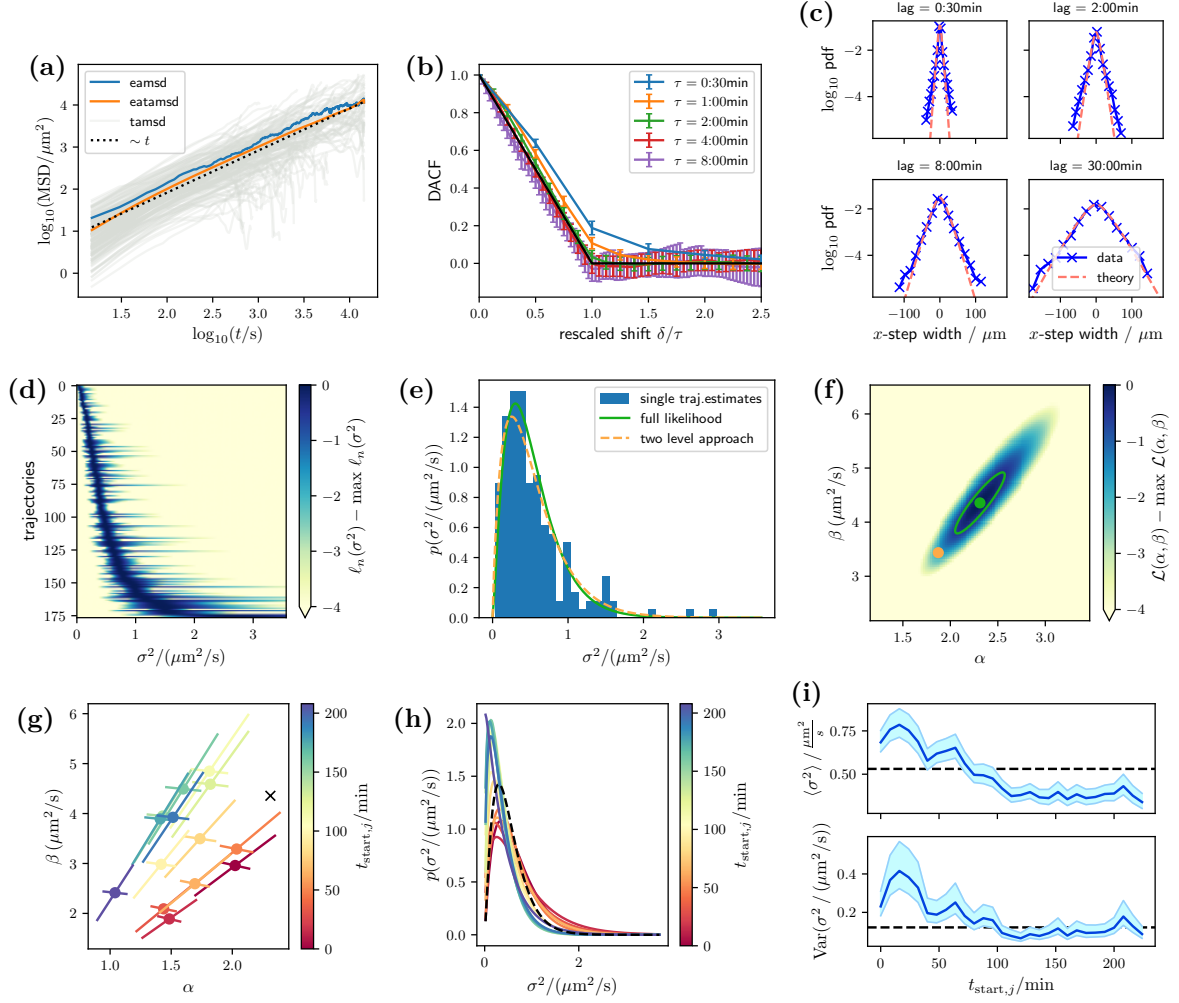

**Figure S5:** Results for dataset with bead diameter of  $61 \mu\text{m}$ . The inference results are obtained using sparse versions of the trajectories with  $\Delta t = 2 \text{ min}$ . The first row shows the preliminary statistical analysis: (a) mean squared displacement, (b) normalized and rescaled displacement autocorrelation function, (c) step-size distributions. The second row shows inference using the full length of each trajectory: (d) single trajectory log-likelihood of  $\sigma^2$ , (e) distribution of single trajectory estimates and inferred heterogeneity, (f) log-likelihood of the heterogeneity parameters. The third row shows results of heterogeneity inference using data within a time window of 16 min: (g) inferred heterogeneity parameter, (h) inferred probability density functions, (i) mean and variance of the inferred distributions.

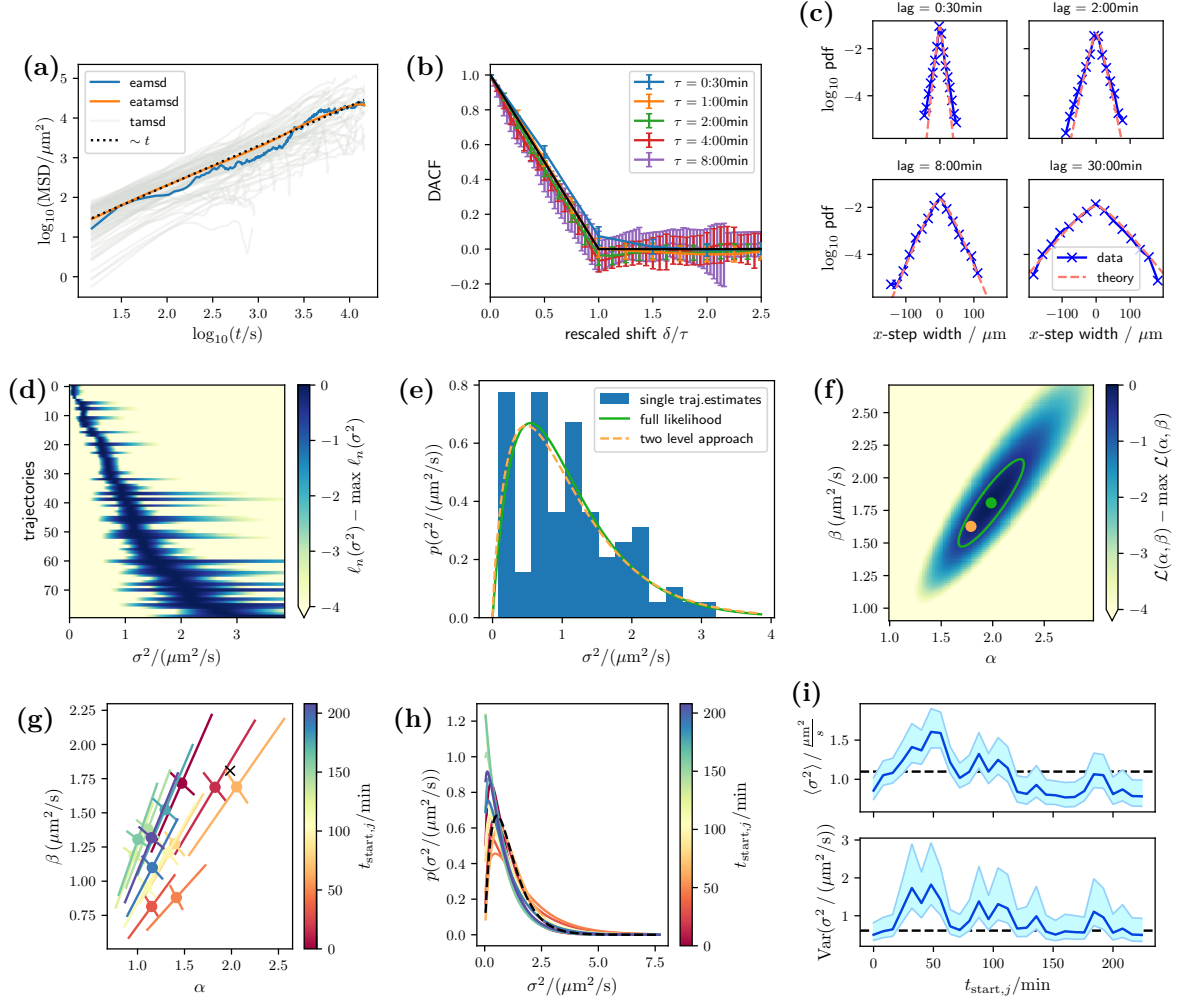

**Figure S6:** Results for dataset with bead diameter of  $100 \mu\text{m}$ . The inference results are obtained using sparse versions of the trajectories with  $\Delta t = 2 \text{ min}$ . The first row shows the preliminary statistical analysis: (a) mean squared displacement, (b) normalized and rescaled displacement autocorrelation function, (c) step-size distributions. The second row shows inference using the full length of each trajectory: (d) single trajectory log-likelihood of  $\sigma^2$ , (e) distribution of single trajectory estimates and inferred heterogeneity, (f) log-likelihood of the heterogeneity parameters. The third row shows results of heterogeneity inference using data within a time window of 16 min: (g) inferred heterogeneity parameter, (h) inferred probability density functions, (i) mean and variance of the inferred distributions.

## S4 Calculation of Hessian matrix

As stated in the main text, the Hessian matrix of the likelihood provides a measure of uncertainty of the maximum likelihood estimates. Here, we sketch a way how to calculate and implement the Hessian matrix for the model used in the paper. Compare also [1].

For ease of notation we define  $\boldsymbol{\theta} := (\alpha, \beta)$  and use  $\kappa, \lambda$  to refer to components of  $\boldsymbol{\theta}$ .

The elements of the Hessian matrix are given by  $\sum_n \partial_\kappa \partial_\lambda \mathcal{L}_n$ . Exploiting the fact that the likelihood is calculated as an integral over  $\sigma^2$  we find that

$$\begin{aligned} \partial_\kappa \partial_\lambda \mathcal{L}_n(\boldsymbol{\theta}) &= \partial_\kappa \partial_\lambda \log \int d\sigma^2 p(\mathbf{T}^n | \sigma^2) q_\Gamma(\sigma^2 | \boldsymbol{\theta}) \\ &= \mathbb{E}_n \left[ \frac{\partial_\kappa \partial_\lambda q_\Gamma(\sigma^2 | \boldsymbol{\theta})}{q_\Gamma(\sigma^2 | \boldsymbol{\theta})} \right] - \mathbb{E}_n \left[ \frac{\partial_\kappa q_\Gamma(\sigma^2 | \boldsymbol{\theta})}{q_\Gamma(\sigma^2 | \boldsymbol{\theta})} \right] \mathbb{E}_n \left[ \frac{\partial_\lambda q_\Gamma(\sigma^2 | \boldsymbol{\theta})}{q_\Gamma(\sigma^2 | \boldsymbol{\theta})} \right], \end{aligned} \quad (\text{S1})$$

where  $\mathbb{E}_n[\cdot]$  denotes an expectation value with respect to  $p(\sigma^2 | \mathbf{T}^n, \boldsymbol{\theta}) = p(\mathbf{T}^n | \sigma^2) q_\Gamma(\sigma^2 | \boldsymbol{\theta}) / p(\mathbf{T}^n | \boldsymbol{\theta})$  and  $q_\Gamma(x)$  denotes the probability density function of a  $\Gamma$ -distribution. Note that the denominator is just the likelihood. The relevant expressions inside the expectation values are:

$$\frac{\partial_\alpha q_\Gamma(x | \boldsymbol{\theta})}{q_\Gamma(x | \boldsymbol{\theta})} = \log \beta - \psi(\alpha) + \log(x) \quad (\text{S2})$$

$$\frac{\partial_\beta q_\Gamma(x | \boldsymbol{\theta})}{q_\Gamma(x | \boldsymbol{\theta})} = \frac{\alpha}{\beta} - x \quad (\text{S3})$$

$$\frac{\partial_\alpha \partial_\beta q_\Gamma(x | \boldsymbol{\theta})}{q_\Gamma(x | \boldsymbol{\theta})} = \frac{1}{\beta} + (\log \beta - \psi(\alpha) + \log x) \left( \frac{\alpha}{\beta} - x \right) \quad (\text{S4})$$

$$\frac{\partial_\alpha \partial_\alpha q_\Gamma(x | \boldsymbol{\theta})}{q_\Gamma(x | \boldsymbol{\theta})} = -\psi^{(1)}(\alpha) + (\log \beta - \psi(\alpha) + \log(x))^2 \quad (\text{S5})$$

$$\frac{\partial_\beta \partial_\beta q_\Gamma(x | \boldsymbol{\theta})}{q_\Gamma(x | \boldsymbol{\theta})} = -\frac{\alpha}{\beta^2} + \left( \frac{\alpha}{\beta} - x \right)^2. \quad (\text{S6})$$

Here,  $\psi(x) = \frac{d}{dx} \log \Gamma(x)$  denotes the digamma function and  $\psi^{(1)}(x) = \frac{d}{dx} \psi(x)$  denotes the polygamma function of order 1.

The expectation value of the constants is trivial. The remaining expectation values can be expressed in terms of modified Bessel functions and their derivatives with respect to the index. In the following,  $K_\nu(x)$  denotes the modified Bessel function of the second kind;  $K'_\nu(x)$  and  $K''_\nu(x)$  are derivatives of  $K_\nu(x)$  with

respect to index  $\nu$ :

$$\mathbb{E}_n[x] = \sqrt{\frac{a_n}{\beta}} \frac{K_{(-1+b_n-\alpha)}(2\sqrt{a_n\beta})}{K_{(b_n-\alpha)}(2\sqrt{a_n\beta})} \quad (\text{S7})$$

$$\mathbb{E}_n[\log x] = \frac{1}{2} \log\left(\frac{a_n}{\beta}\right) - \frac{K'_{(b_n-\alpha)}(2\sqrt{a_n\beta})}{K_{(b_n-\alpha)}(2\sqrt{a_n\beta})} \quad (\text{S8})$$

$$\mathbb{E}_n[x^2] = a_n \frac{K_{(2-b_n+\alpha)}(2\sqrt{a_n\beta})}{\beta K_{(b_n-\alpha)}(2\sqrt{a_n\beta})} \quad (\text{S9})$$

$$\mathbb{E}_n[x \log x] = \sqrt{\frac{a_n}{\beta}} \frac{K_{(1-b_n-\alpha)}(2\sqrt{a_n\beta}) \log\left(\frac{a_n}{\beta}\right) - 2K'_{(-1+b_n-\alpha)}(2\sqrt{a_n\beta})}{2 K_{(b_n-\alpha)}(2\sqrt{a_n\beta})} \quad (\text{S10})$$

$$\mathbb{E}_n[(\log x)^2] = \frac{1}{4} \left( \log\left(\frac{a_n}{\beta}\right) \right)^2 + \frac{-\log\left(\frac{a_n}{\beta}\right) K'_{(b_n-\alpha)}(2\sqrt{a_n\beta}) + K''_{(b_n-\alpha)}(2\sqrt{a_n\beta})}{K_{(b_n-\alpha)}(2\sqrt{a_n\beta})}. \quad (\text{S11})$$

$a_n$  and  $b_n$  are defined in the Appendix of the main text.

## References

- [1] J. Albrecht, M. Opper, and R. Großmann. Inferring parameter distributions in heterogeneous motile particle ensembles: A likelihood approach for second order langevin models. 2024.
- [2] R. Großmann, L. S. Bort, T. Moldenhawer, M. Stange, S. S. Panah, R. Metzler, and C. Beta. Non-Gaussian displacements in active transport on a carpet of motile cells. *Phys. Rev. Lett.*, 132(8):088301, 2024. doi:[10.1103/PhysRevLett.132.088301](https://doi.org/10.1103/PhysRevLett.132.088301).
- [3] R. K. Sadhu, M. Luciano, W. Xi, C. Martinez-Torres, M. Schröder, C. Blum, M. Tarantola, S. Villa, S. Penič, A. Iglič, C. Beta, O. Steinbock, E. Bodenschatz, B. Ladoux, S. Gabriele, and N. S. Gov. A minimal physical model for curvotaxis driven by curved protein complexes at the cell's leading edge. *Proc. Natl. Acad. Sci.*, 121(12):e2306818121, 2024. doi:[10.1073/pnas.2306818121](https://doi.org/10.1073/pnas.2306818121).
